# Supplementary material for: Ultrafast quantum dynamics in $\mathbf{\mathrm{SrTiO_3}}$ under impulsive THz radiation
Source: arXiv:2408.12421 source file (2024-08-22)
Supplement: Supplementary file 1 [file supporting_information.tex]

\newpage
\thispagestyle{empty}
\onecolumngrid
\appendix

\section{Machine-learned potential}\label{flare}

For the machine-learned interatomic potential (MLIP), we choose FLARE~\cite{Vandermause2020}, as it provides active learning for efficient data generation and fast inference times~\cite{trill}. 
The active learning explored different temperatures and volumes to create a transferable potential.
At each of 100, 300 and 500 K, the system was simulated for 200 ps at the DFT-relaxed lattice parameter as well as \(\pm2\)\% strain for a total of 1.8 ns of dynamics.
We used a timestep of 2 fs and a thermostat damping time of 200 fs with LAMMPS's~\cite{lammps22} default Nosé–Hoover thermostat.
The procedure is shown in \figurename~\ref{timeline}, where the bottom panel shows how the maximum atomic uncertainty was used to determine whether to compute forces, energy and stress with DFT and retrain the potential.
Before each change in temperature, the uncertainty threshold was doubled.
 The DFT calculations are performed at the PBE level of theory, using the open source software Quantum ESPRESSO \cite{Giannozzi_2009}.
 We employ a plane-wave cutoff of 80 Ry, and a k-point grid of $\mathrm{6\times6\times8}$ for the 20-atom cell. We adopt the pseudopotentials suggested by the SSSP efficiency library \cite{prandini2018precision}. 

\begin{figure}
    \centering
    \includegraphics[scale=0.2]{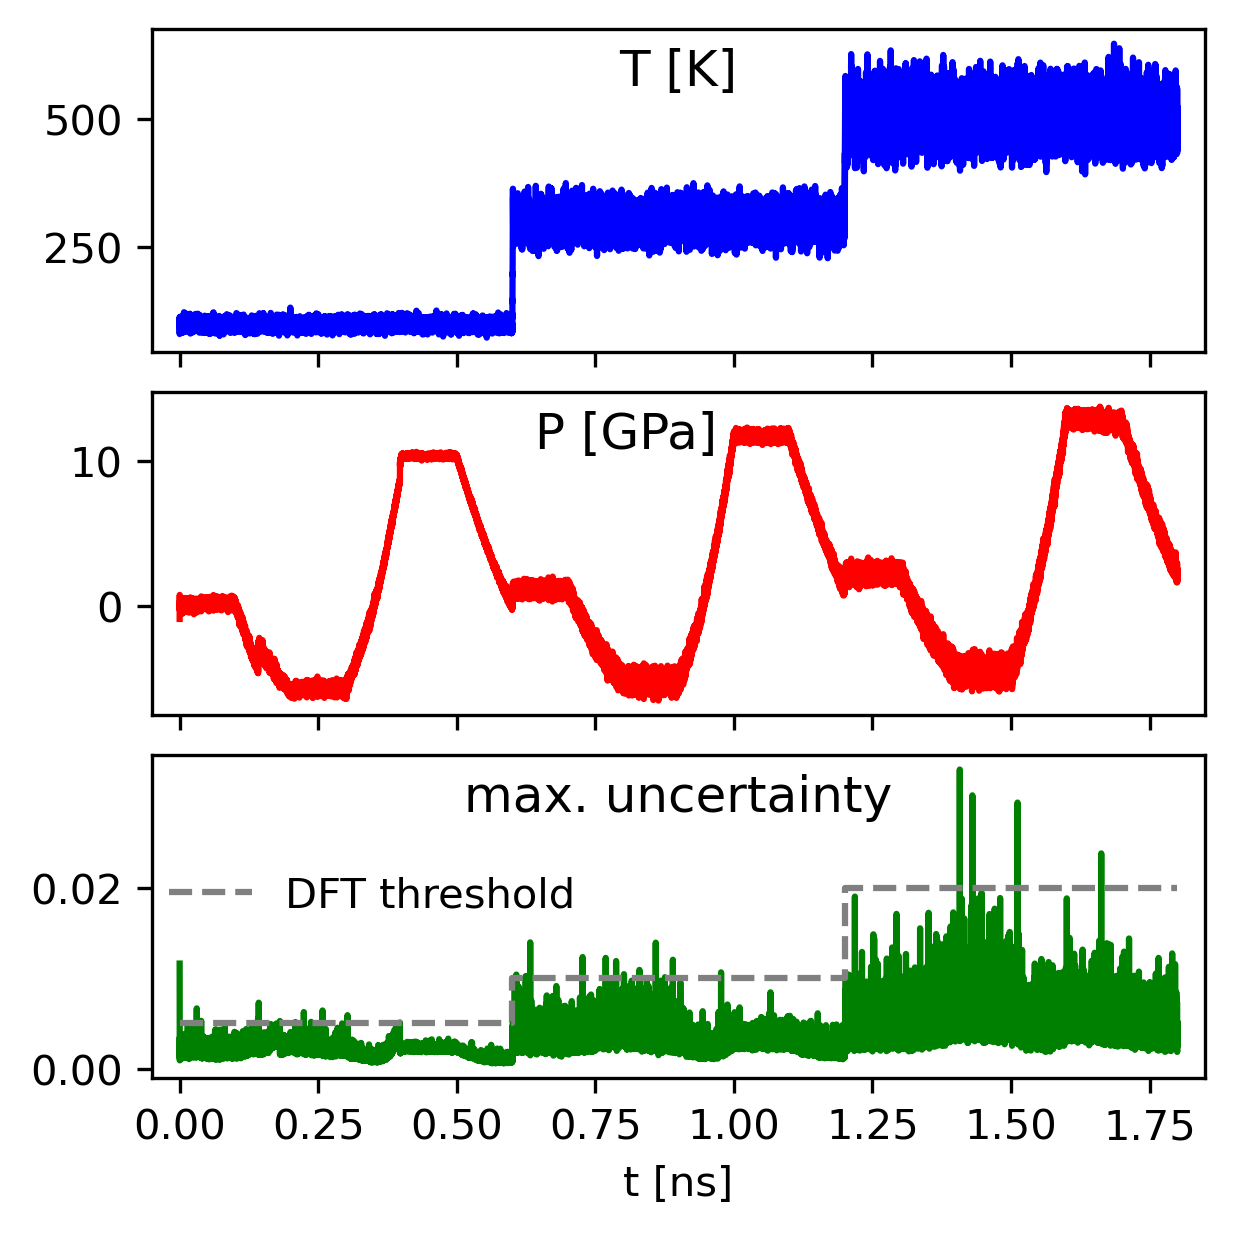}
    \caption{Active learning run with FLARE. At each temperature, the cell is first kept at the DFT-relaxed lattice parameter for 100 ps, then the lattice parameter is linearly increased by 2\% over 100 ps, where it is kept constant for another 100 ps. Over the next 100 ps, the lattice parameter is decreased to 2\% less than the initial, relaxed value, where it is kept for another 100 ps. Finally, the lattice parameter is returned to the relaxed value over the final 100 ps.}
    \label{timeline}
\end{figure}

The double well potential energy given by the MLIP is in good agreement with the density functional theory results (see Fig. \ref{PES_SPM}). In order to check the accuracy of the MLIP, we calculate also the equation of state, both for the cubic and the tetragonal cells, reported in Fig \ref{eos}. 
Being short-ranged, the MLIP is not able to capture long-range effects in the force constants. As a result, it does note fully capture the splitting between the high-frequency longitudinal and transverse optical degenerate modes \cite{PhysRevB.1.910,COCHRAN1962447,RevModPhys.73.515, Rivano2023}. This error in the phonon frequencies is not expected to significantly affect the dynamics, as the SPM is characterized by a much lower frequency.

\begin{figure}
    \centering
    \includegraphics[scale=0.5]{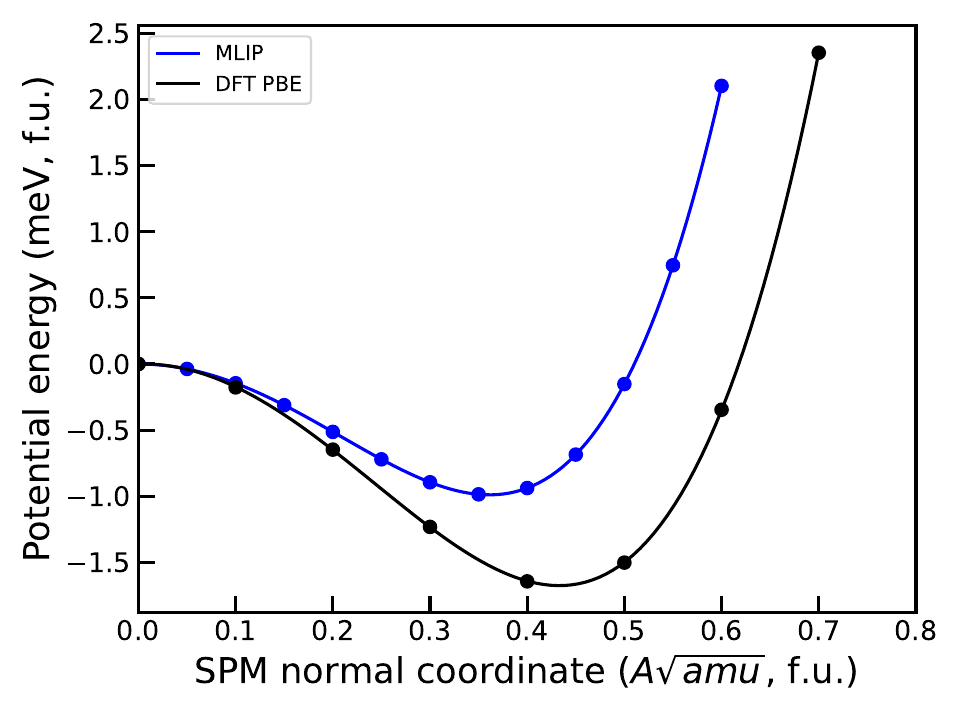}
    \caption{Potential energy surface of the SPM, calculated both with DFT-PBE (black line) and MLIP (blue line).}
    \label{PES_SPM}
\end{figure}

\begin{figure}
    \centering
    \begin{subfigure}{0.49\textwidth}
        \includegraphics[scale=0.5]{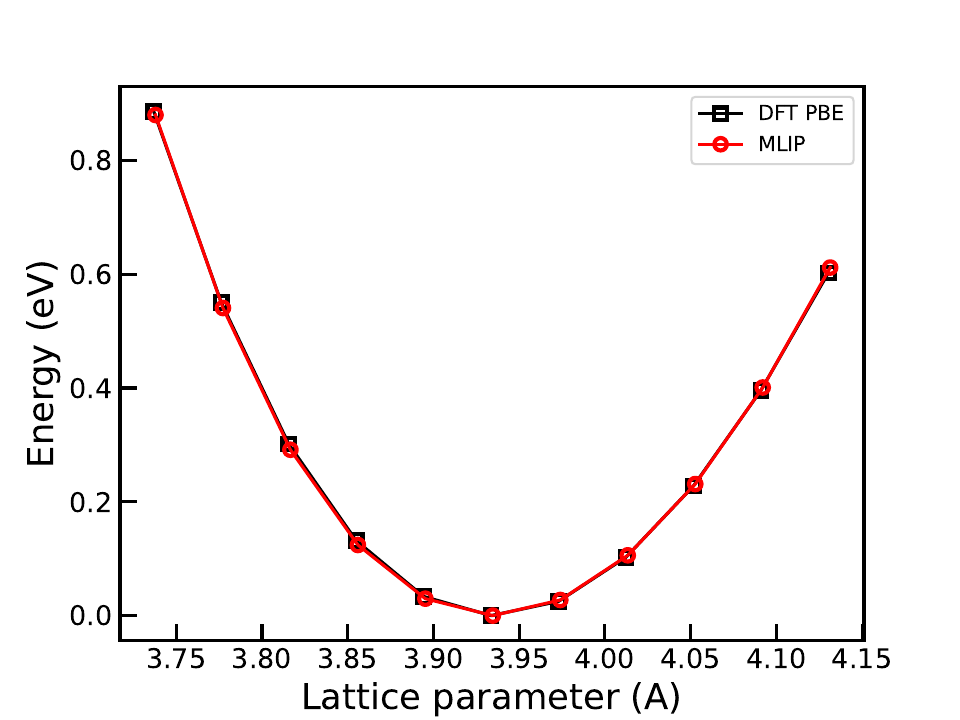}
        \label{Cubic}
    \end{subfigure}
    \begin{subfigure}{0.49\textwidth}
        \includegraphics[scale=0.5]{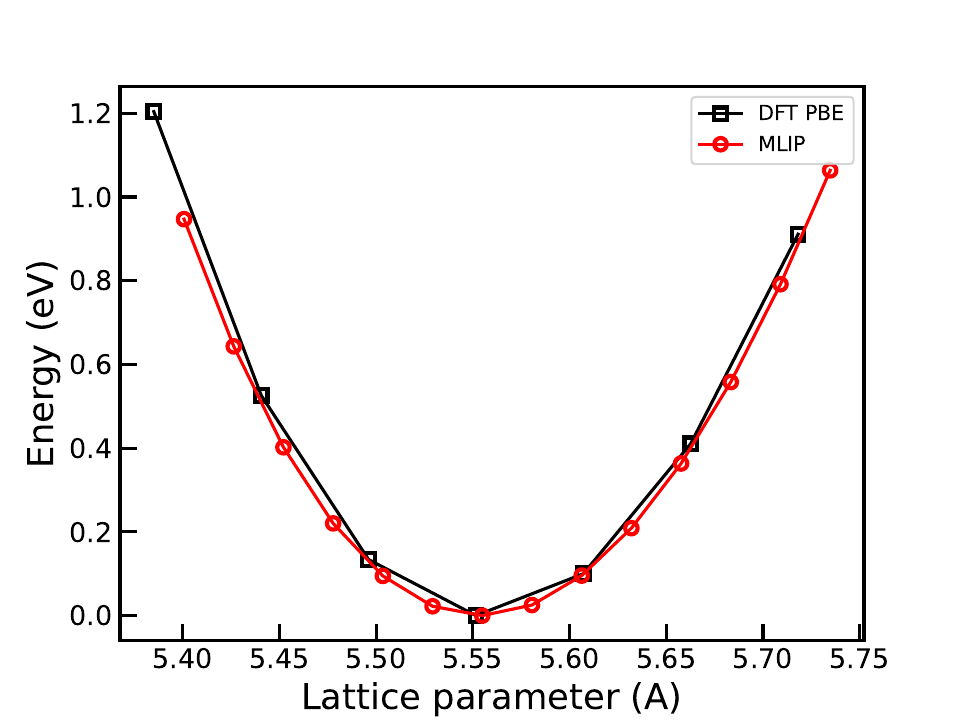}
        \label{Tetragonal}
    \end{subfigure}    
    \caption{This figure compares the equation of state for the cubic STO cell (Panel a) and the tetragonal 20-atom cell (Panel b), calculated with DFT PBE calculations (black line) with that obtained through MLIP (red line).  }
    \label{eos}
\end{figure}

\section{Pulse shape, dielectric screening and Born effective charges}
To simulate phonon upconversion, we use a single-cycle pulse of the following shape, which reproduces the main features of the pulse applied in Ref. \cite{Kozina2019}:
\begin{equation}
f(t) = -A\ \frac{t}{\sigma}e^{-\frac{t^2}{2\sigma^2}+\frac{1}{2}}
\end{equation}
This pulse reaches its maximum at $t=\sigma$, with $|f(\sigma)|=A$.
Furthermore, its Fourier transform is
\begin{equation}
F(\omega) = -iA\ \sigma^2 \omega\ e^{-\frac{1}{2}\omega^2\sigma^2+\frac{1}{2}}
\end{equation}
which peaks at $\omega_0=1/\sigma$, corresponding to a frequency of
\begin{equation}
f = \frac{1}{2\pi \sigma}
\end{equation}
The investigation of the THz field induced ferroelectric transition, instead, employ a Gaussian pulse of equation
\begin{equation}
    f(t) = A\cos(\omega_0 (t-t_0))e^{-\frac{(t-t_0)^2}{2\sigma^2}}\ .
\end{equation}
The value of $\sigma$ employed in the simulations is 468 fs. 
The Fourier transform of this pulse reads
\begin{equation}
    F(\omega)=\frac{\sigma}{2} \Bigl( e^{-\frac{1}{2}(\omega-\omega_0)^2\sigma^2} + e^{-\frac{1}{2}(\omega+\omega_0)^2\sigma^2 }\Bigr)\ .
\end{equation}
If $\omega_0>\sigma$, this pulse is peaked at $\omega=\omega_0$, with spread $1/\sigma$.
The forces on the atom due to the electric field are obtained as
\begin{equation}
    \mathbf{f}_a= \frac{1}{\varepsilon_{eff}}\ \mathbf{Z}_a\cdot \mathbf{\mathcal{E}}\ ,
\end{equation}
where $\mathbf{\mathcal{E}}$ is the external electric field, $e$ is the electron charge, $\varepsilon_{eff}$ is the dielectric constant and $\mathbf{Z}_a$ are the Born effective charge tensors. The effective charges are calculated through Density funtional perturbation theory (DFPT), using the same parameters as specified in Section \ref{flare}. Their value for the different atomic species is reported in Table \ref{Zeff}.
\begin{table}[h]
    \centering
    \begin{tabular}{c|c|c|c|}
           & $\mathrm{Z^*_{xx}}$ & $\mathrm{Z^*_{yy}}$ & $\mathrm{Z^*_{zz}}$\\ \hline\hline
        Ti & 7.338 & 7.338 & 7.338\\
        Sr & 2.549 & 2.549 & 2.549\\
        $\mathrm{O_1}$ & -2.024 & -5.845 & -2.024 \\
        $\mathrm{O_2}$ & -2.024 & -2.024&  -5.845\\
        $\mathrm{O_3}$ & -5.845 & -2.024 & -2.024\\
    \end{tabular}
    \caption{Born effective charges for the cubic STO unit cell, computed through DFPT.}
    \label{Zeff}
\end{table}
Here we employ the screening model proposed in Refs. \cite{PhysRevB.85.045134, PhysRevLett.129.167401} 
\begin{equation}
    \varepsilon_{eff} = \frac{1+\sqrt{\varepsilon_{DFPT}}}{2}\ ,
\end{equation}
with $\varepsilon_{DFPT}=6.31$.

\section{Existence of a metastable ferroelectric state}\label{C}
\begin{figure}[h]
    \centering
    \begin{subfigure}{0.32\textwidth}
        \includegraphics[scale = 0.35]{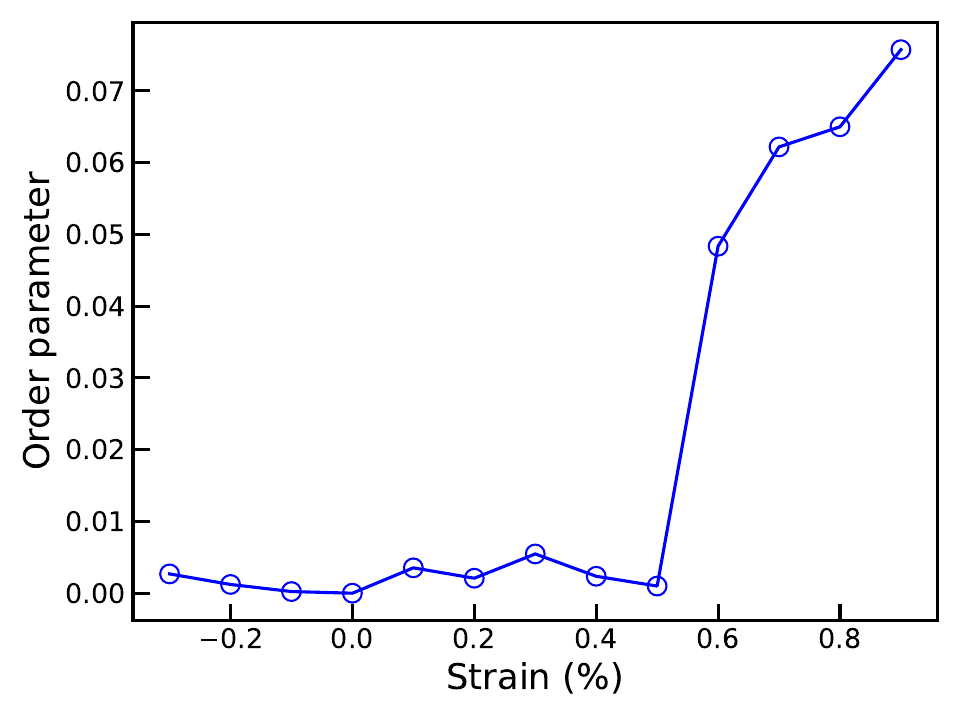}
        \caption{Order parameter}
        \label{op}
    \end{subfigure}
    \begin{subfigure}{0.32\textwidth}
        \includegraphics[scale = 0.35]{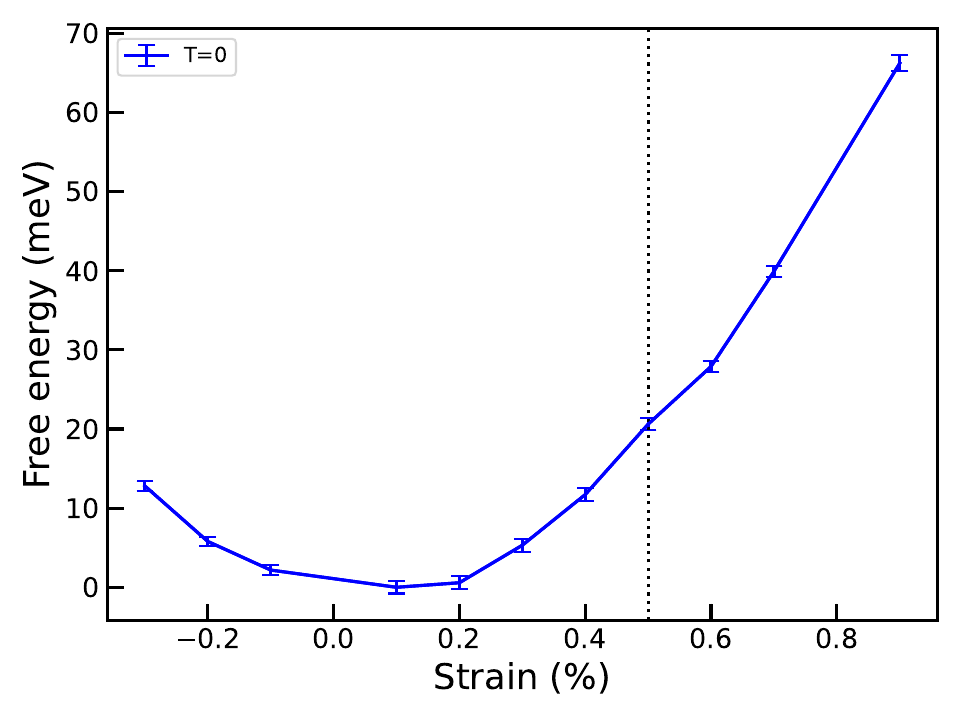}
        \caption{Free energy surface}
        \label{fe}
    \end{subfigure}
    \begin{subfigure}{0.32\textwidth}
        \includegraphics[scale = 0.35]{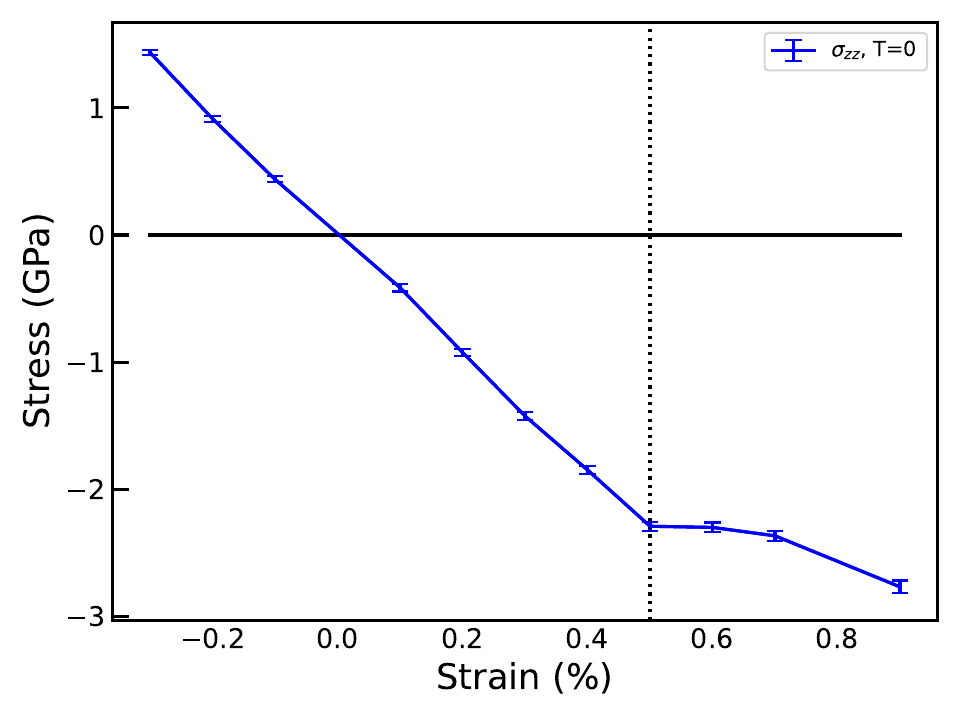}
        \caption{Stress}
        \label{st}
    \end{subfigure}
    \caption{Panel (a) shows the order parameter defined in Eq. \ref{op_eq} as a function of the isotropic strain. Panel (b) shows the zz component of the stress and the free energy (upper and lower part respectively) as a function of the strain. The stress is defined such that a negative value corresponds to tensile stress.   }
    \label{op-fe}
\end{figure}
The transition into a permanent ferroelectric state implies the presence a metastable state in the free energy surface, corresponding to a vanishing strain condition. In order to verify whether such a local minimum exists, we perform SSCHA calculations at 0K for a 20-atom STO cell with isotropic strains ranging from -0.3\% to 0.9\%. The order parameter describing the ferroelectric transition is chosen as
\begin{equation}\label{op_eq}
    OP = \Bigl|\sum_i r^{crystal}_{iz}(\varepsilon) - \sum_i r^{crystal}_{iz}(\varepsilon=0) \Bigr|\ .
\end{equation}
Here, $r^{crystal}_{iz}(\varepsilon)$  denotes the crystal coordinate of the i-th atom along the z-direction following a SSCHA relaxation calculation at a strain $\varepsilon$. This parameter is expected to remain approximately constant for a paraelectric system due to inversion symmetry and to change when this symmetry is broken. Fig. \ref{op} represents the order parameter as a function of the strain. We can clearly see that $\varepsilon=0.6\%$ marks the onset of a ferrolectric transition. This transition corresponds to a change in the free energy profile and the slope of the stress-strain curve (represented in Fig.\ref{fe} and Fig.\ref{st} respectively). Remarkably, after the trasition, both the stress-strain curve and the free energy profile continue to change monotonically, making it impossible for the stress to vanish and for the free energy to exhibit a local minimum as a function of the strain. This result implies that there does not exist a ferroelectric metastable state with a periodicity equal to that of a 20-atom STO cell. The strain at which the transition occurs is largely overestimated relative to experiment due to the use of the PBE functional for training the MLIP. As mentioned in the main text, this functional tends to underestimate the energy barrier height, thus favoring the paraelectric phase. The predicted transition strain can be corrected using a one-dimensional model of a particle in a double-well potential, given by the equation~\cite{PhysRevResearch.4.033020}:
\begin{equation}
\frac{V}{V_0} = -2\Bigl(\frac{x}{x_0}\Bigr)^2 + \Bigl(\frac{x}{x_0}\Bigr)^4\ .
\end{equation}
The parameters of the model, namely the height $V_0$ of the energy barrier and the position $x_0$ of the minima, are tuned based on the RPA calculations from Ref. \cite{PhysRevMaterials.7.L030801}, with values $V_0 = 5$ meV (f.u.) and $x_0 = 0.42 \AA \sqrt{u}$ (f.u.). Fig. \ref{model} shows both the order parameter (solid line) and the pressure (dashed line) obtained by solving the one-dimensional model with SSCHA. The parametrization of the model with RPA calculations (red line) yields a transition strain of 0.1\% and a transition pressure of a few hundred kilobars. The accuracy of the model can be evaluated by comparing the predictions obtained from the model parameterized using DFT-PBE calculations (blue line) with the full SSCHA calculation using the MLIP parameterized on PBE calculations in Fig. \ref{st}. The results show very good agreement, suggesting that a full SSCHA calculation witha MLIP parametrixed on RPA calculations would lead a similar result to that obtained with the model (red curve).
\begin{figure}
    \centering
    \includegraphics[scale=0.5]{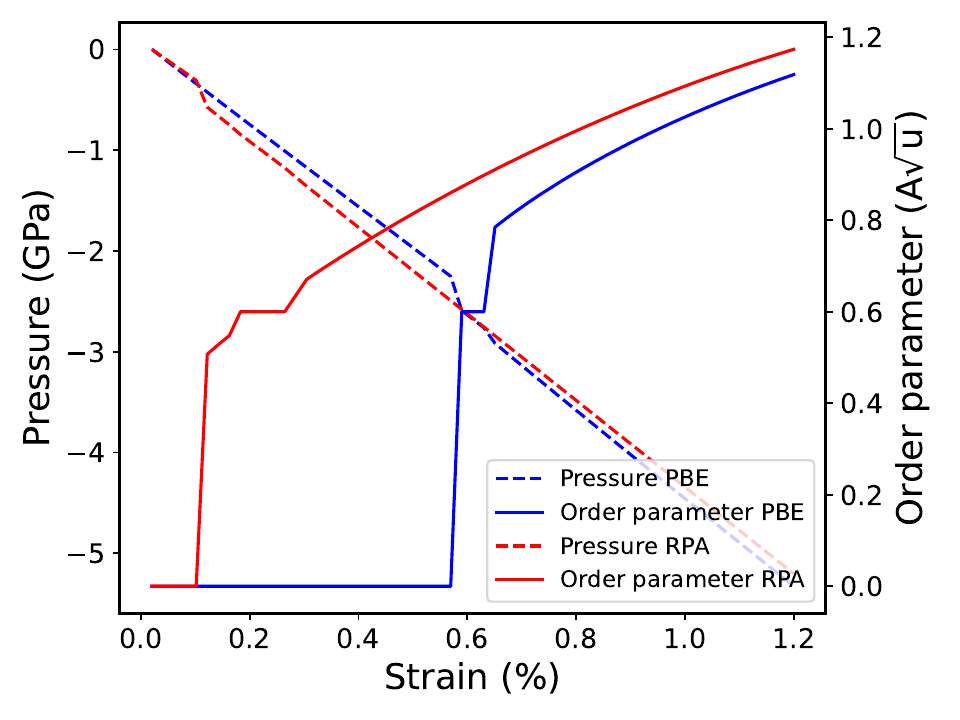}
    \caption{The solid lines represent the order parameter, indicated by the relaxed position of the particle in the 1D potential, for both the RPA (red) and PBE (blue) parametrizations. The dashed lines depict the pressure acting on the sample, with negative pressure indicating positive stress. }
    \label{model}
\end{figure}
